# Supplementary material for: Ultrafast dephasing of light in strongly scattering GaP nanowires
Source: arXiv:1102.3408 source file (2011-02-16)
Supplement: Supplementary file 1 [file abb_supplementary.pdf]

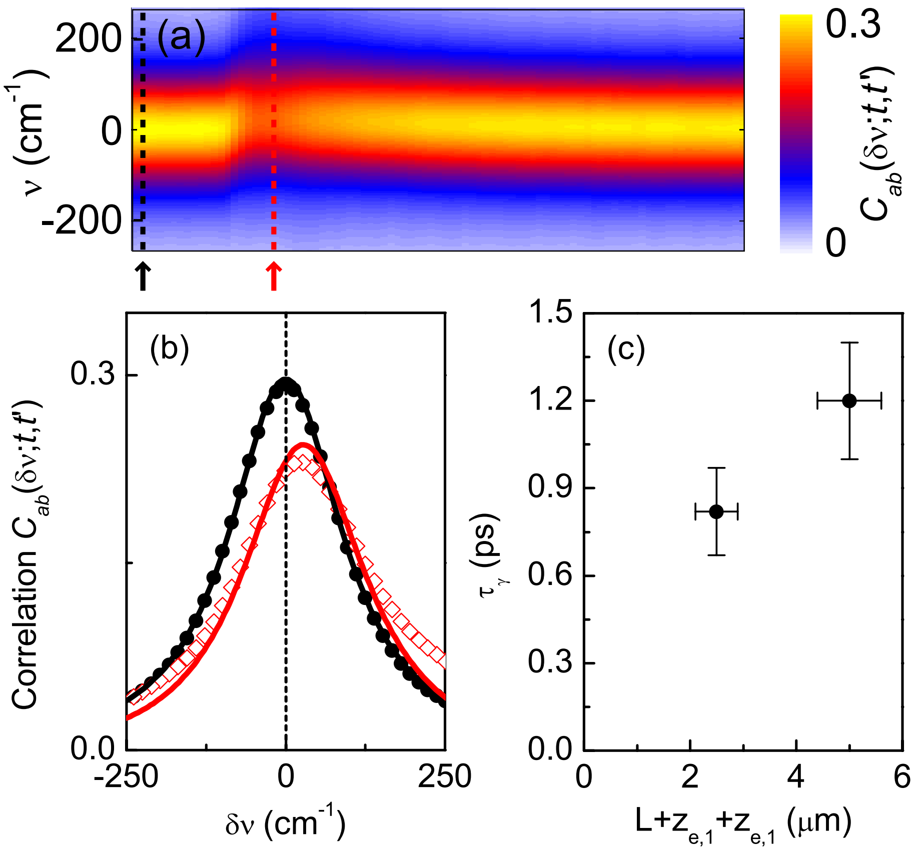


FIG. 1: (color online) (a) Map of experimental correlation $C_{ab}(\nu; t, t')$ for sample 1. (b) Cross sections of (a) at delay times of $-3$ ps (dots, black),and 1 ps (diamonds, red). Lines represent fits, without (black) and with (red line) dephasing model with $\tau_\gamma = 0.82{\pm}0.15$ ps and $D = 13.6{\pm}2$ m$^2$/s. (c) Values of $\tau_\gamma$ against effective slab thickness $L + z_{e,1} + z_{e,2}$ for samples 1 and 2.

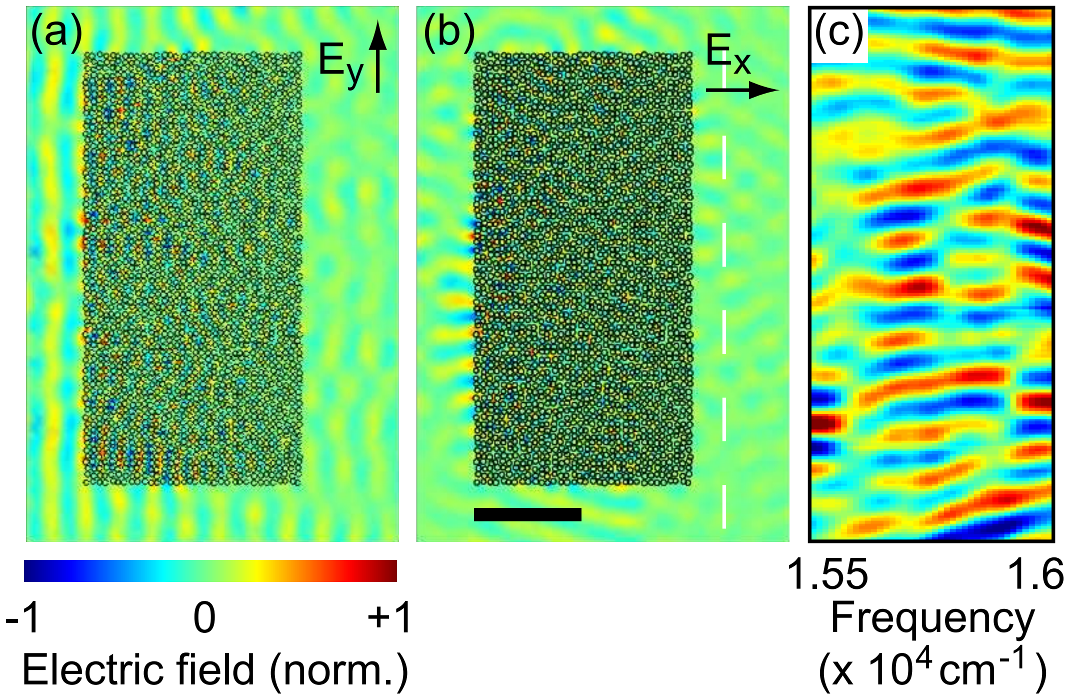


FIG. 2: COMSOL model of a 2D random medium. Scattering cylinders have a diameter of 100 nm with random variations of $\pm$10 nm; filling factor is 50%. (a,b) Calculated electric fields from numerical finite-element model (COMSOL) for a random slab of scatterers for polarizations parallel $E_y$ (a) and perpendicular (b) $E_x$ to the incident light. Scale bar, 2 $\mu$m. (c) Electric field $E_x$ against frequency, 0.5 $\mu$m from the exit surface of the slab (dashed line in b).
